# Supplementary material for: A Unified View of Evaluation Metrics for Structured Prediction
Source: arXiv:2310.13793 source file (2023-10-20)
Supplement: Supplementary file 1 [file coref.tex]

\subsection{MUC}
 The widely used MUC metric for coreference resolution \citep{vilain-etal-1995-model} is a link-based metric  that reports precision, recall, and $\rm F_1$ for the links denoting the coreference relationships between mentions.\footnote{~The MUC metric is not to be confused with the metrics presented in \S\ref{subsec:tf} for scoring template filling on MUC-4.}  MUC computes its recall as 
\begin{equation}
    \recall_{\rm MUC} = \frac{\sum_{r\in R} (\left|r\right| - \left|p_P(r)\right|)}{\sum_{r\in R} (\left| r\right| - 1)},
\end{equation}
where $p_P(r)$ is the partition of $r$ with $P$, the predicted set of entities. Note that the nominator can be written as $\sum_{r \in R}\left( \sum_{I \in p_P(r)} \left|I\right| - 1 \right)$: thus we can define the number of shared coreference links as a similarity function between entities:
\begin{equation}
    \phi_{\rm link}(X, Y) = \max\{0, \left| X \cap Y \right| - 1\}.
\end{equation}
Then we have the following using unconstrained matching:
\begin{equation}
    \recall_{\rm MUC} = \recall^{\sim}_\texttt{entities}[\phi_{\rm link}].
\end{equation}
Precision / ${\rm F}_1$ can be defined similarly.

\subsection{$B^3$}
$B^3$ \citep{bagga1998algorithms} tries to solve two problems with MUC: first, MUC's failure to reward correct identification of singleton entities (since it counts \emph{links} only), and second, its intrinsic bias in favor of system outputs containing fewer entities. However, it has numerous problems of its own \citep{luo-2005-coreference, moosavi-strube-2016-coreference, luo2016evaluation}. For instance, \citet{luo2016evaluation} note that if a given reference mention is repeated across multiple predicted entities, $B^3$ will award credit for each one.

In contrast to MUC, $B^3$ focuses on \emph{mentions}. Suppose $P_m$ and $R_m$ are the predicted and reference entities that contain mention $m$, and suppose $c(P_m)$ is the number of correct mentions in $P_m$, i.e.:
\begin{equation}
c(P_m) = |P_m \cap R_m| = \phi_3(P_m, R_m)
\end{equation}
$B^3$ computes $m$-specific precision and recall as:
\begin{align}
    \text{precision}(m) &= \frac{c(P_m)}{|P_m|}\label{eq:b3-mention-precision} \\
    \text{recall}(m) &= \frac{c(P_m)}{|R_m|}\label{eq:b3-mention-recall}
\end{align}
It then computes overall precision and recall as a weighted average over all mentions $m$:
\begin{align}
    \text{precision}_\text{total} &= \sum_{m \in M} w_m \cdot \text{precision}(m)\label{eq:b3-total-precision} \\
    \text{recall}_\text{total} &= \sum_{m \in M} w_m \cdot \text{recall}(m)\label{eq:b3-total-recall}
\end{align}
where $M$ is the set of all predicted mentions.\footnote{This is the ``informal'' formulation of $B^3$ described in \citet{bagga1998algorithms}. See their paper, as well as \citet{moosavi-strube-2016-coreference} for alternative, equivalent formulations.} \citeauthor{bagga1998algorithms} use a weighted average to allow for heavier weighting of mentions that are ``more important,'' according to whatever notion of importance may be applicable.\footnote{The notion of mention informativity, discussed in \S\ref{sec:discussion}, would be one example.} However, the standard practice is to use the same weight for all $m$.

Although $B^3$ is a mention-level metric, it can nonetheless be viewed as computing a score over an unconstrained alignment ($A^\sim$) between \emph{entities}. The question, then, is what the entity similarity function is. To start, consider that $c(P_m)$ is the same for all mentions $m \in P_m \cap R_m$, as is the denominator of Eqs. \ref{eq:b3-mention-precision} and \ref{eq:b3-mention-recall}. Thus, Eqs. \ref{eq:b3-mention-precision} and \ref{eq:b3-mention-recall} as a whole are equivalent for all mentions $m \in P_m \cap R_m$. This in turn implies that there will be $|P_m \cap R_m|$ copies of $\text{precision}(m)$ in the sum of Eq. \ref{eq:b3-total-precision} and the same number of copies of $\text{recall}(m)$ in the sum of Eq. \ref{eq:b3-total-recall}. The trouble is that, owing to the per-mention normalization in Eqs. \ref{eq:b3-mention-precision} and \ref{eq:b3-mention-recall}, we cannot write Eqs. \ref{eq:b3-total-precision} and \ref{eq:b3-total-recall} as $\precision$- and $\recall$-normalized sums (respectively) of the same similarity function between entity pairs. Rather, we must define different similarities for precision and for recall:
\begin{align}
    \phi_\texttt{Entity-R}(P,R) &= \frac{|P \cap R|}{|R|} \sum_{m \in P \cap R} w_m\label{eqn:b3-entity-r-similarity} \\
    \phi_\texttt{Entity-P}(P,R) &= \frac{|P \cap R|}{|P|} \sum_{m \in P \cap R} w_m\label{eqn:b3-entity-p-similarity}
\end{align}
Eqs. \ref{eq:b3-total-precision} and \ref{eq:b3-total-recall} can then be expressed as sums of Eqs. \ref{eqn:b3-entity-r-similarity} and \ref{eqn:b3-entity-p-similarity}, respectively, over all entity pairs.
