# Supplementary material for: A Unified View of Evaluation Metrics for Structured Prediction
Source: arXiv:2310.13793 source file (2023-10-20)
Supplement: Supplementary file 2 [file todolist.tex]

\begin{enumerate}
    \item Why alignment metric can be a unified view of SP? We have to justify this is widely used in evaluating structure prediction tasks. 
    \item The atomic operator should have a positive range. Why?
\end{enumerate}
